# Supplementary material for: Ensemble Spectral Prediction (ESP) Model for Metabolite Annotation
Source: arXiv:2203.13783 source file (2022-03-25)
Supplement: Supplementary file 1 [file SI_Fig_3steps.tex]

\begin{figure*}%[tbhp]
\centering
\includegraphics[width=.95\linewidth]{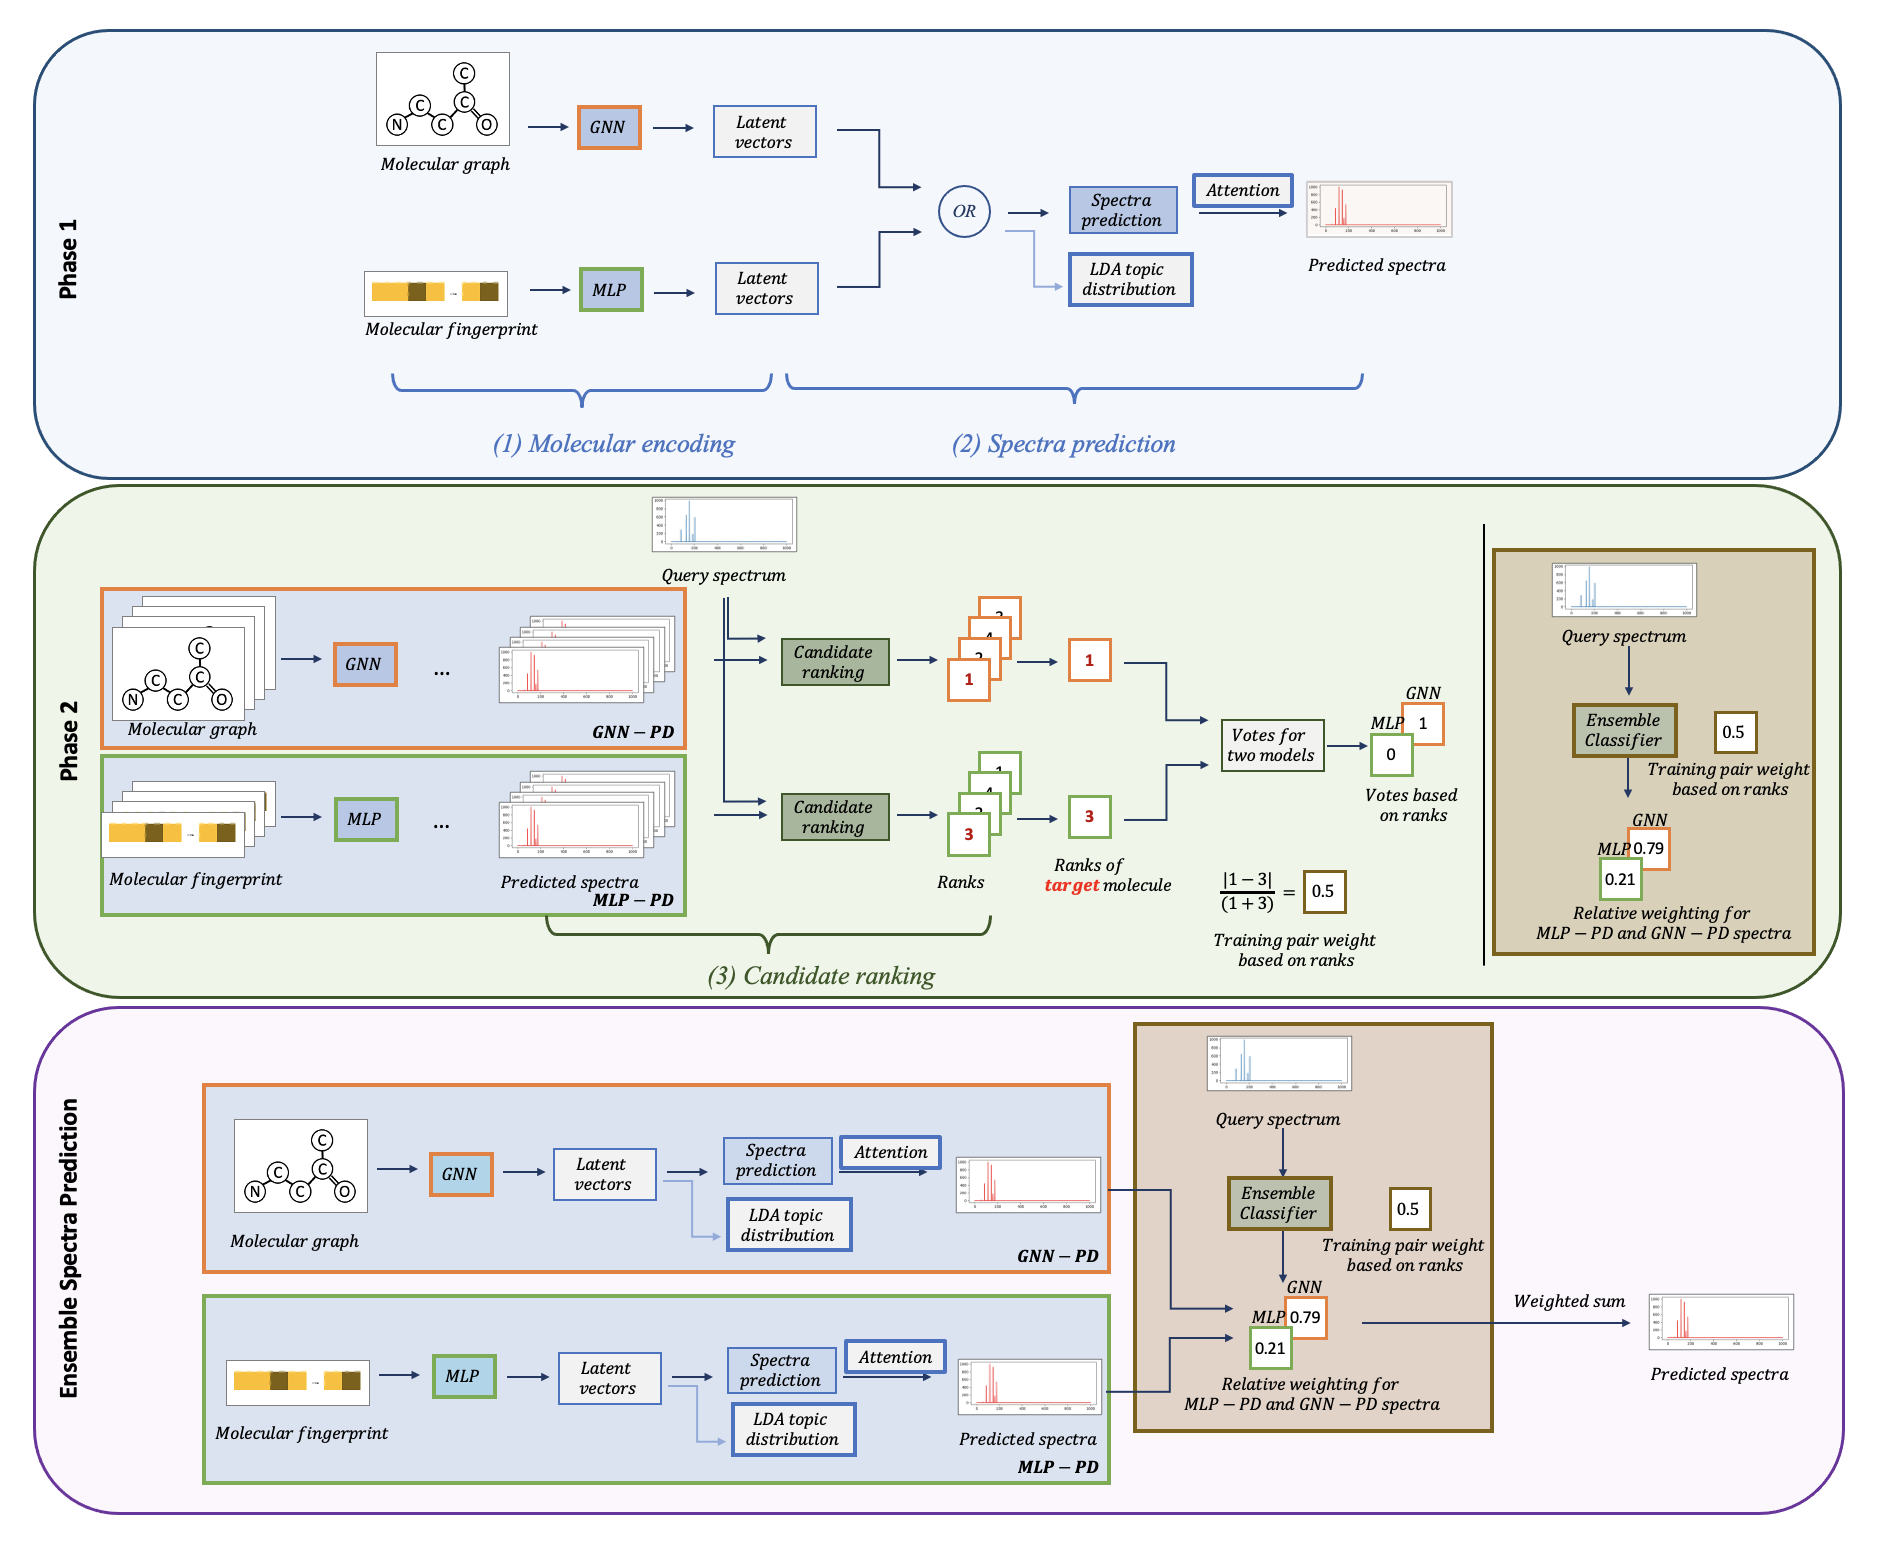}
 \caption{\textbf{Two phases in ensemble spectra prediction modeling.}\textbf{Step 1,} molecular encoding and spectra prediction enhancement, where we use MLP and GNN models to encode different molecular information, together with peak dependency enhanced spectra prediction via attention and multi-tasking on predicting LDA topic distribution; \textbf{Step 2, }training ensemble scoring model, we compare the rank of spectra prediction from GNN and MLP encoding on candidate ranking problem for query spectra in the training set to predict a score on weighing the two models. Note that ESP focus on solving the three subproblems of metabolite annotation: GNN and MLP models in Step 1 focus on \textbf{Problem 1} molecular encoding; attention and multi-tasking on LDA topic distribution prediction in Step 1 focus on \textbf{Problem 2} spectra encoding; ensemble scoring based on ranks of target molecule from two models focus on \textbf{Problem 3} candidate ranking.}
\label{fig:si_3step}
\end{figure*}
