# Supplementary material for: Ensemble Spectral Prediction (ESP) Model for Metabolite Annotation
Source: arXiv:2203.13783 source file (2022-03-25)
Supplement: Supplementary file 2 [file SI_Fig_mix.tex]

\begin{figure*}%[tbhp]
\centering
\includegraphics[width=.95\linewidth]{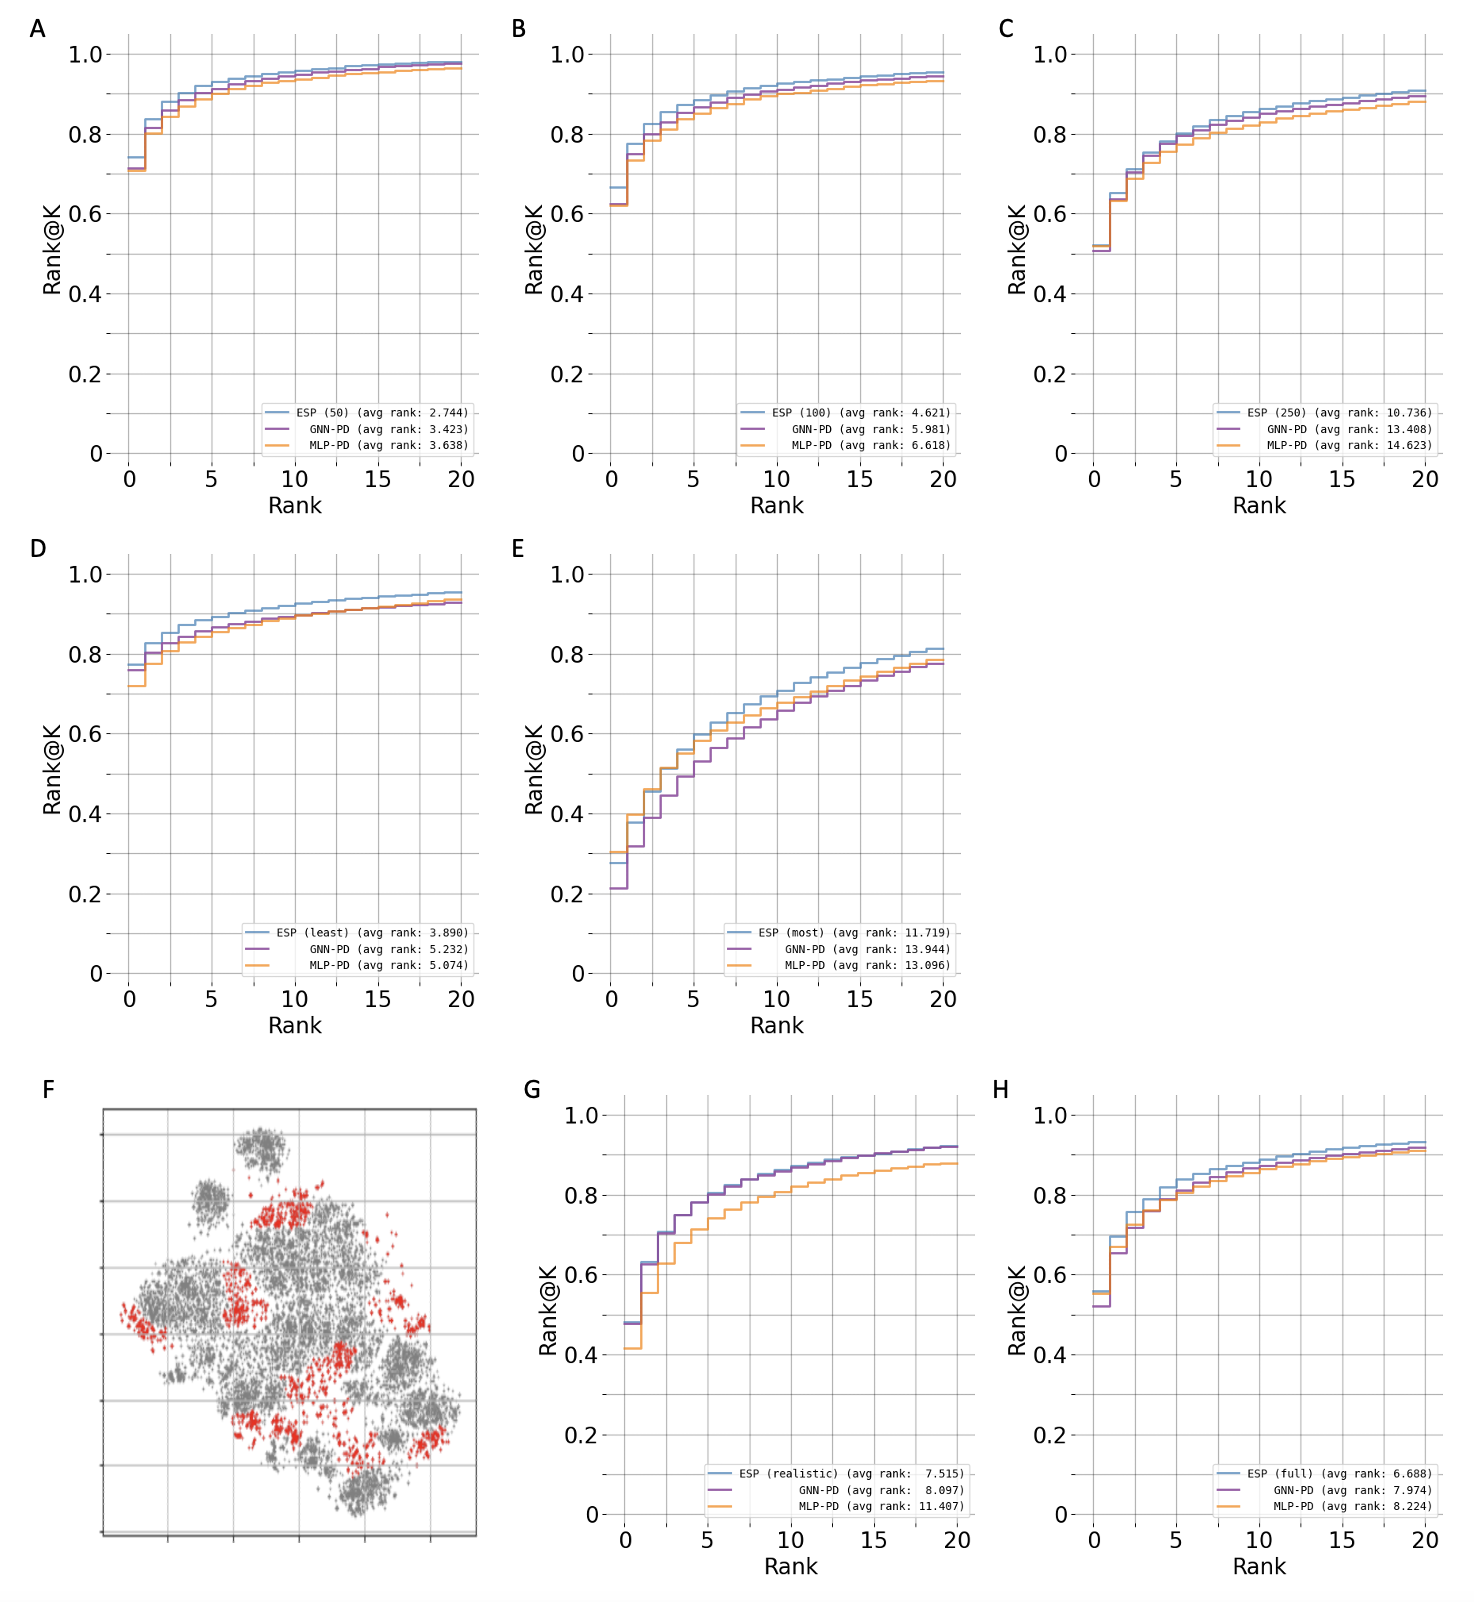}
\caption{Candidate ranking performances (Rank@K) for different settings for ESP model (except for F), comparing with GNN-PD and MLP-PD models. A), B), C) are 50-molecule, 100-molecule, 250-molecule candidate set, respectively, D) Least similar candidate set, E) Most similar candidate set, F) Realistic split t-SNE plot (Grey clusters for training, red clusters for test), G) Realistic split set, H) Full positive data set.}
\label{fig:mix}
\end{figure*}
