# Supplementary material for: Ensemble Spectral Prediction (ESP) Model for Metabolite Annotation
Source: arXiv:2203.13783 source file (2022-03-25)
Supplement: Supplementary file 3 [file SI_Fig_molsize.tex]

\begin{figure}%[tbhp]
\centering
\includegraphics[width=.9\linewidth]{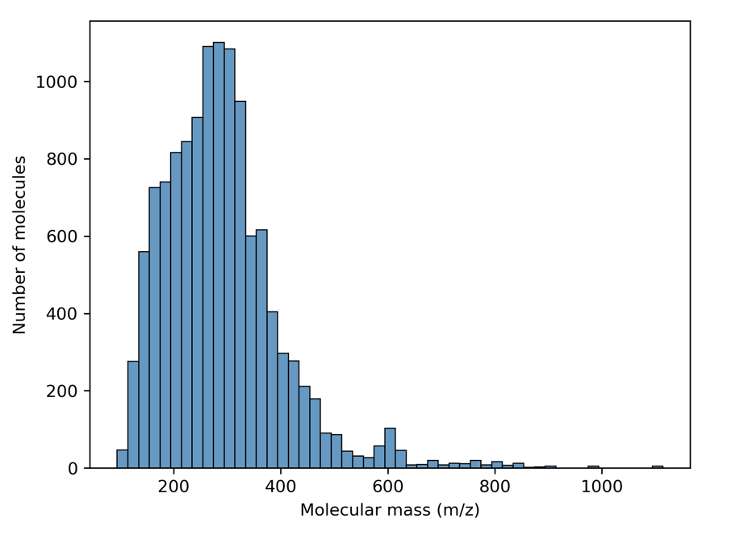}
 \caption{Histogram of molecular mass in test set (x-axis)}
\label{fig:si_molsize}
\end{figure}
